# Supplementary material for: EL PASSO: Privacy-preserving, Asynchronous Single Sign-On
Source: arXiv:2002.10289 source file (2020-06-03)
Supplement: Supplementary file 1 [file appendix.tex]

%!TEX root = ../main.tex
%=========================================================

\appendix

\section{Cryptographic Construction}
\label{sec:appendix}

We present the detailed cryptographic protocols in \sysname.

\sysname uses NIZK to assert knowledge and relations over discrete logarithm values.
We represent these non-interactive zero-knowledge proofs with the notation introduced by Camenisch~\etal~\cite{camenisch1997proof}
\[
{\rm NIZK}\{(x,y,\dots): \textrm{statements about } x, y, \dots\}
\]
which denotes proving in zero-knowledge that the secret values $(x,y,\dots)$ satisfy the statements after the colon; the statement and all other values are public.

\subsection{Anonymous Credential Scheme}
\label{sec:appendix:credential}

In this section, we present the construction of the anonymous credential scheme with \ps and NIZK protocol which can be implemented with Schnorr protocol with Fiat-Shamir heuristic~\cite{RFC8235}.

In \sysname, a credential is generated over a number of attributes.
In Cred.Issue, some attributes are kept unknown to the authority while in Cred.Prove the credential holder can select a different set to hide from the verifier.
Assume there are totally $n$ attributes certified by the \ps credential, denoted by $a_1, ..., a_n$.
For the sake of reading, we let the hidden attributes in Cred.Issue be the first $m$ ($m$ < $n$) attributes and the hidden attributes in Cred.Prove be the first $m'$ ($m'$ < $n$, $m'$ can be different from $m$) attributes.

The construction of anonymous credential is as follows.

\begin{description}[leftmargin=1em, labelindent=0em]
	\setlength\itemsep{.3em}
	\item[\newdef{Cred.Setup($1^\lambda$)}{$\mathit{pp}$}] run by the authority and output the public parameter
	\[
	pp \leftarrow (p, \mathbb{G}_1, \mathbb{G}_2, \mathbb{G}_T, e)
	\]
	where $p$ is a large prime number, $\mathbb{G}_1, \mathbb{G}_2, \mathbb{G}_T$ are bilinear groups of type 3, and $e$ is the pairing function.

	\item[\newdef{Cred.KeyGen($\mathit{pp}$)}{$sk, pk$}]
	run by the authority and output:
	\[
	sk \leftarrow g^x
	\]
	\[
	pk \leftarrow (g, g^{y_1}, g^{y_2}, ..., g^{y_n}, \tilde{g}, \tilde{g}^{y_1}, \tilde{g}^{y_2}, ..., \tilde{g}^{y_n})
	\]
	where $n$ is total number of attributes and $g, \tilde{g}$ are group generators randomly selected from $\mathbb{G}_1$ and $\mathbb{G}_2$, respectively.
	$x, y_1, y_2, ..., y_n$ are randomly generated from $\mathbb{F}$.

	\item[\newdef{Cred.Issue($sk, M_h,M_p,\phi$)}{$\sigma$}]
	\textsf{Cred.Issue} is composed of three algorithms.
	Here, instead of committing all the attributes as stated by Pointcheval and Sanders~\cite{pointcheval}, only hidden attributes are committed by the user while the commit of public attributes is simulated by the authority.

	\vspace{2mm}

	\begin{description}
		\item\newdef{Cred.PrepareBlindSign($pk, M_h, \phi$)}{$d, \Lambda, \phi$}
		The user first commits hidden attributes $M_h = a_1, ..., a_m$ by computing
		\[
		\Lambda_1 \leftarrow g^d \prod_{i = 1}^{m} (g^{y_i})^{a_i}
		\]
		(where $d$ is randomly selected from $\mathbb{F}$).
		The user then compute $\Lambda_2$ to be the NIZK proof of the attributes $M_h$ and the correctness of $\Lambda_1$.
		\[
		\Lambda_2 \leftarrow {\rm NIZK}\{(d, a_1, ..., a_m): \phi \}
		\]
		Finally, output $\Lambda \leftarrow (\Lambda_1, \Lambda_2)$.

		\item\newdef{Cred.Sign($sk, M_p, \Lambda,\phi$)}{$\tilde{\sigma}$}
		Let $(\Lambda_1, \Lambda_2) = \Lambda$.
		The authority first verifies the NIZK proof $\Lambda_2$ against $\phi$ following the NIZK  verification protocol.
		After that, the authority appends the public attributes to $\Lambda_1$ to simulate the commitment of all the attributes.
		\[
		\Lambda_1' = \Lambda_1 \prod_{i = m+1}^{n} (g^{y_i})^{a_i}
		\]
		Then the authority generates the PS signature credential.
		\[
		\tilde{\sigma} \leftarrow (g^u, (sk~\Lambda_1')^u)
		\]
		(where $u$ is randomly selected by the authority from $\mathbb{F}$).

		\item\newdef{Cred.Unblind($d, \tilde{\sigma}$)}{$\sigma$}
		Let $(\tilde{\sigma}_1, \tilde{\sigma}_2) = \tilde{\sigma}$.
		The user unblinds the PS signature by outputting
		$\sigma \leftarrow (\tilde{\sigma}_1, \tilde{\sigma}_2 / \tilde{\sigma}_1^d)$

	\end{description}

	\item[\newdef{Cred.Prove($pk, M_p, M_h, \sigma, \phi'$)}{$M_p, \Theta, \phi'$}]
	Letting \\ $(\sigma_1, \sigma_2) = \sigma$, the prover will first randomize the credential $\sigma$ into $\sigma'$ by
	\[
	\sigma' \leftarrow (\sigma_1^{t}, (\sigma_1~\sigma_2^{t})^{r})
	\]
	(where $t, r$ are randomly selected from $\mathbb{F}$ by the prover).
	This ensures $\sigma'$ is indistinguishable from $\sigma$.
	Then, letting $(\sigma_1', \sigma_2')$ $ = \sigma'$, the prover calculates a committed message $\Theta_1$ over hidden attributes $M_h = a_1, ..., a_{m'}$ and $t$.
	\[
	\Theta_1 \leftarrow \tilde{g}^x \prod_{i = 0}^{m'} (\tilde{g}^{y_i})^{a_i} \tilde{g}^t
	\]
	(where $\tilde{g}^x$ is from the authority's public key and $t$ is randomly picked from $\mathbb{F}$).
	Then the prover computes the NIZK proof $\Theta_2$ for the attributes $M_h$ and the correctness of $\Theta_1$.
	\[
	\Theta_2 \leftarrow {\rm NIZK}\{(a_1, ..., a_{m'}, t): \phi'\}
	\]
	Finally, output $\Theta \leftarrow (\sigma', \Theta_1, \Theta_2)$.

	\item[\newdef{Cred.Verify($pk, M_p, \Theta, \phi'$)}{$b$}]
	Let $(\sigma', \Theta_1, \Theta_2) = \Theta$ and $(\sigma_1', \sigma_2') = \sigma'$.
	The verifier first verifies the NIZK proof $\Theta_2$ against $\phi'$ following NIZK verification protocol and then calculates $lhs$ and $rhs$ as
	\[
	lhs \leftarrow e(\sigma_1', \Theta_1) \; ; \; rhs \leftarrow e(\sigma_2', \tilde{g})
	\]
	Then the verifier obtains $b \leftarrow 1$ if $rhs$ is equal to $lhs$ and otherwise $b \leftarrow 0$.
\end{description}

\subsection{Reliable Identity Retrieval}

In this section, we present the construction of \textsf{ProveID} and \textsf{VerifyID} when reliable identity retrieval is enabled.

\begin{description}[leftmargin=1em, labelindent=0em]
	\setlength\itemsep{.3em}
	\item[\newdef{ProveID($pk, \sigma, \gamma, \mathit{info}, tp, \mathit{domain}, y$)}{$\Theta, \phi'$}]
	In addition to the process as defined in the \textsf{Cred.ProveID} in \Cref{sec:appendix:credential}, there are two additional elements to prove, the identity retrieval token $E$ and user ID $\zeta$ as defined in \Cref{sec:construction}.

	Therefore, after user invokes \textsf{Cred.Prove}, there will be additional elements in $\Theta$ and $\phi'$:
	\begin{itemize}
		\item $\Theta$ will also carry $E$ and $\zeta$.
		\item $\phi'$ will also contain the statement about the correctness of $E$ and $\zeta$; therefore, the NIZK proof in $\Theta$ will accordingly be extended.
	\end{itemize}

	\item[\newdef{VerifyID($pk, M_p, \Theta, \phi', \mathit{domain}, y$)}{$b$}]
	Besides running \textsf{Cred.Verify}, the RP will also verify the correctness of $E$ and $\zeta$.
\end{description}

\subsection{Multi-device Support}

In multi-device support, since there is only one attribute $s_{new}$ to certify, the algorithms \textsf{Cred.PrepareBlindSign}, \textsf{Cred.Sign}, and \textsf{Cred.Unblind} can be simplified as follow.

	\begin{description}
	\item\newdef{Cred.PrepareBlindSign($pk_{dev}, s_{new}, \phi$)}{$d, \Lambda, \phi$}
	The user commits $s_{new}$ by computing
	\[
	\Lambda_1 \leftarrow g^d (g^{y_{dev}})^{s_{new}}
	\]
	(where $d$ is randomly selected from $\mathbb{F}$ and $g^{y_{dev}}$ is from the public key $pk_{dev}$).
	The the user then compute $\Lambda_2$ to be the NIZK proof of $\Lambda_1$.
	\[
	\Lambda_2 \leftarrow {\rm NIZK}\{(d, s_{new}): \phi \} ; \phi \leftarrow \Lambda_1 = g^d (g^{y_{dev}})^{s_{new}}
	\]
	Finally, output $\Lambda \leftarrow (\Lambda_1, \Lambda_2)$.

	\item\newdef{Cred.Sign($sk, M_p, \Lambda,\phi$)}{$\tilde{\sigma}$}
	Let $(\Lambda_1, \Lambda_2) = \Lambda$.
	The IdP first verifies the NIZK proof $\Lambda_2$ against $\phi$ following the NIZK Schnorr verification protocol.
	Then the IdP generates the PS signature credential.
	\[
	\tilde{\sigma} \leftarrow (g^u, (g^{x_{dev}}~\Lambda_1)^u)
	\]
	where $u$ is randomly selected by the authority from $\mathbb{F}$.

	\item\newdef{Cred.Unblind($d, \tilde{\sigma}$)}{$\sigma$}
	Let $(\tilde{\sigma}_1, \tilde{\sigma}_2) = \tilde{\sigma}$.
	The user unblinds the PS signature by outputting $\sigma \leftarrow (\tilde{\sigma}_1, \tilde{\sigma}_2 / \tilde{\sigma}_1^d)$.
\end{description}
